# Supplementary material for: Xenos: Dataflow-Centric Optimization to Accelerate Model Inference on Edge Devices
Source: arXiv:2302.00282 source file (2023-02-01)
Supplement: Supplementary file 1 [file appendix.tex]

\onecolumn
\section*{A. Resource Cost} 
\label{sec-full-resource}
\begin{figure}[!htbp]
\vspace{-0.5cm}
	\centering
	\subfigure[MobileNet L2 Cost]{
		\label{Ml2-1} 
		\includegraphics[width=1.6in]{./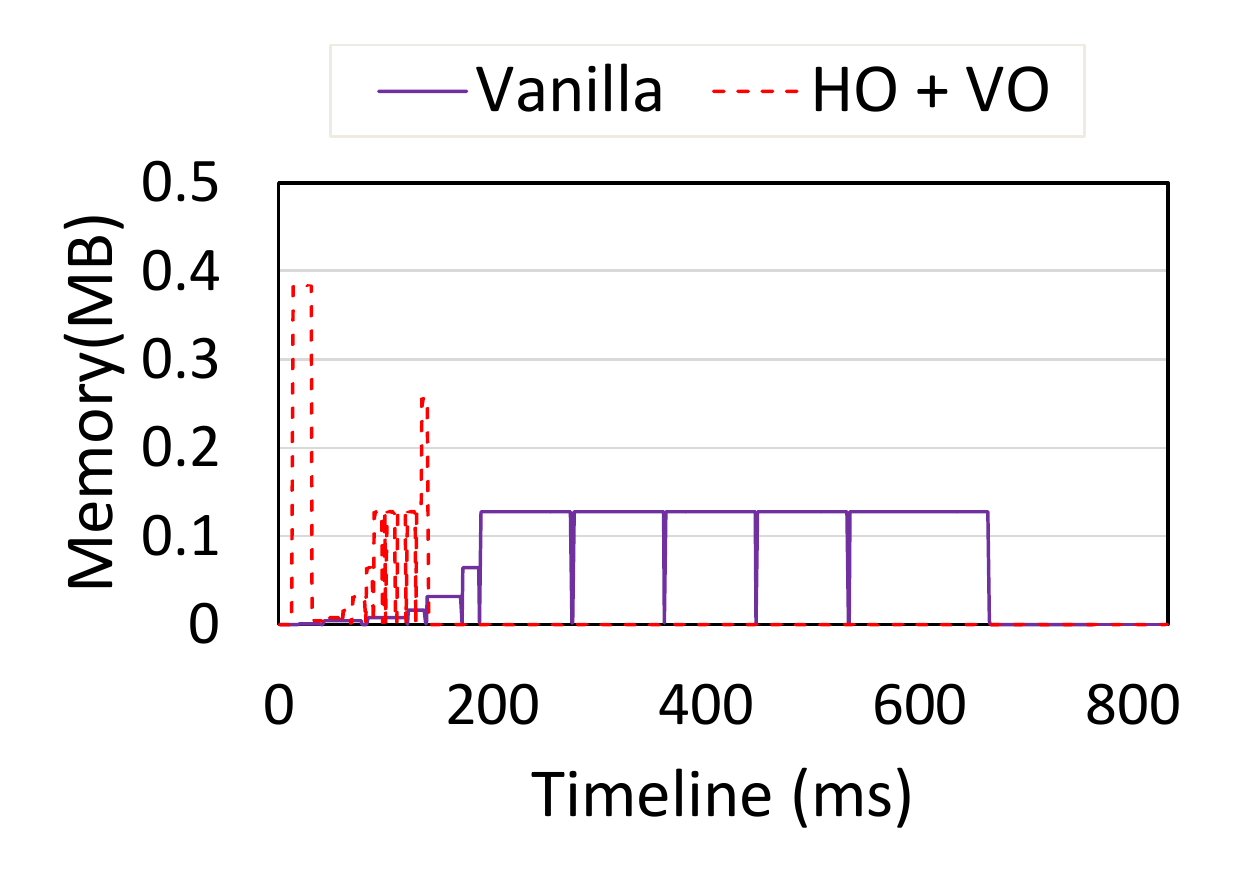}
	}
	\subfigure[MobileNet SRAM Cost]{
    	\label{Msr-1} 
    	\includegraphics[width=1.6in]{./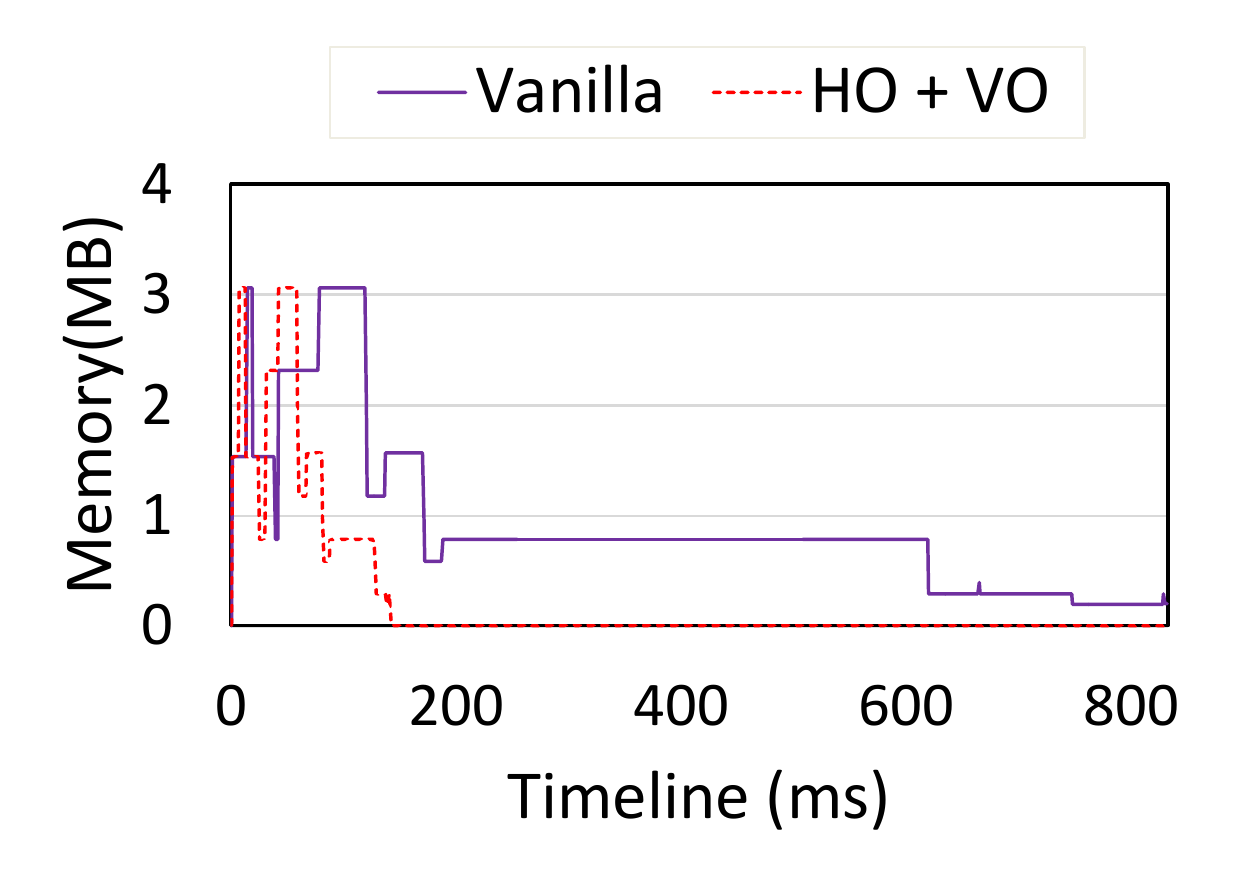}
	}
	\subfigure[MobileNet DDR Cost]{
		\label{Mddr-1} 
		\includegraphics[width=1.6in]{./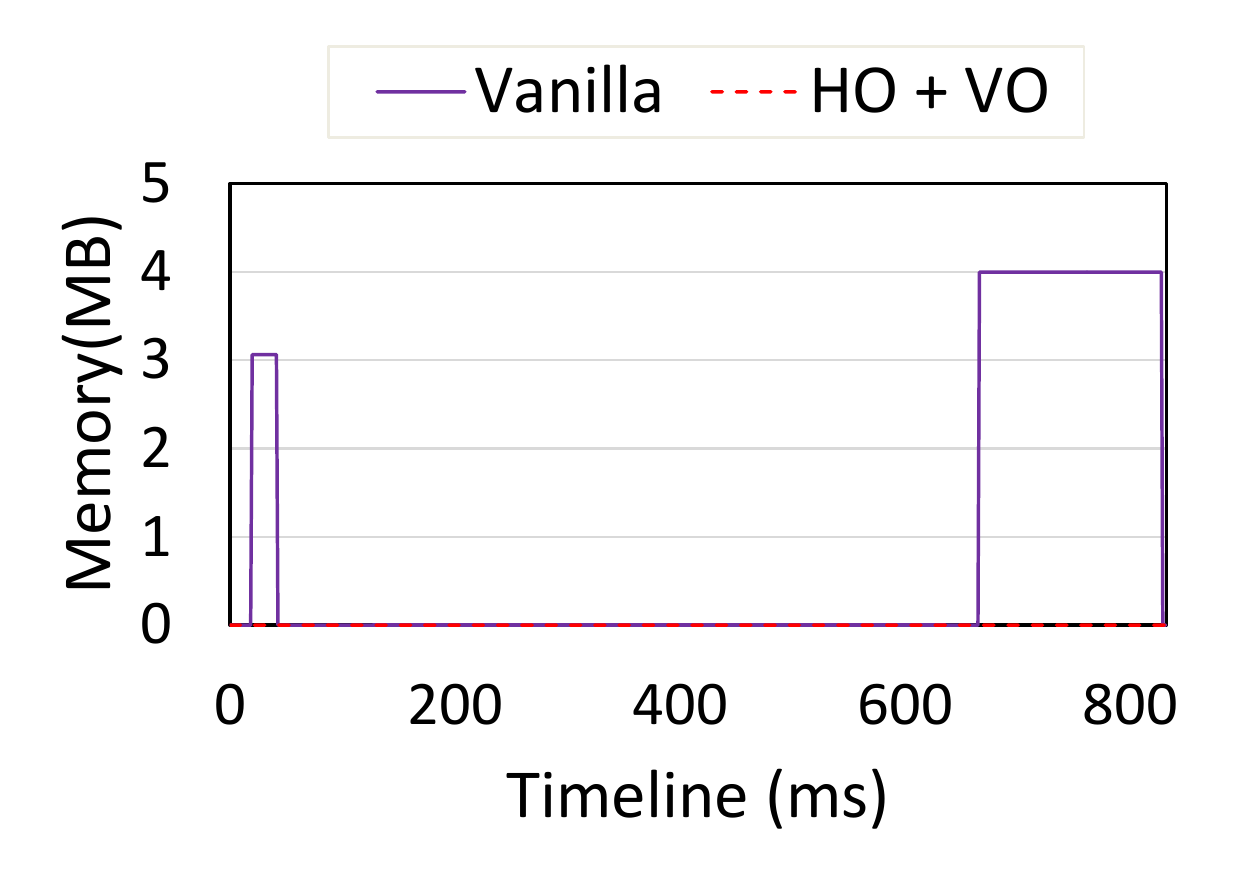}
	}
	\subfigure[MobileNet Total Memory Cost]{
    	\label{Mtotal-1} 
    	\includegraphics[width=1.6in]{./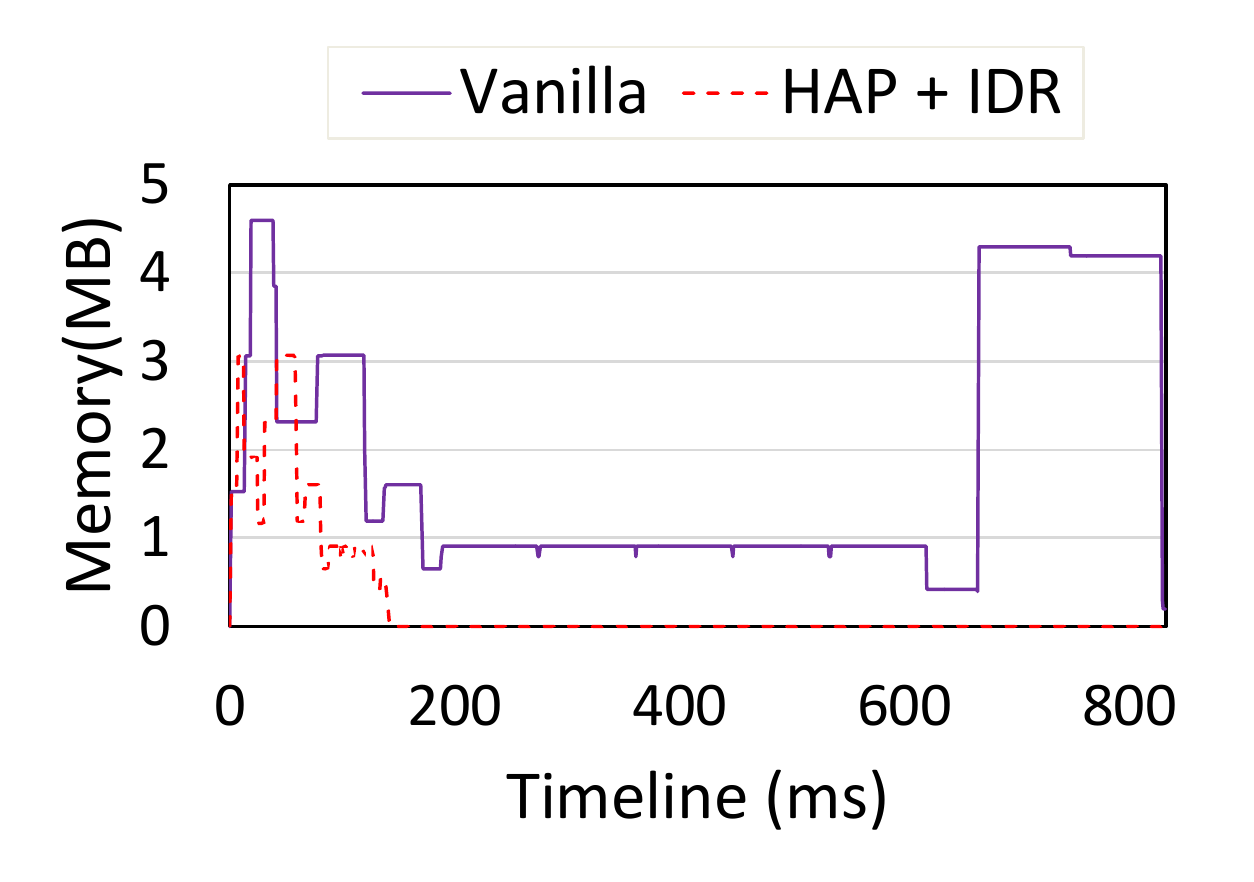}
	} \\[-2ex]
	\subfigure[SqueezeNet L2 Cost]{
		\label{Sl2-1} 
		\includegraphics[width=1.6in]{./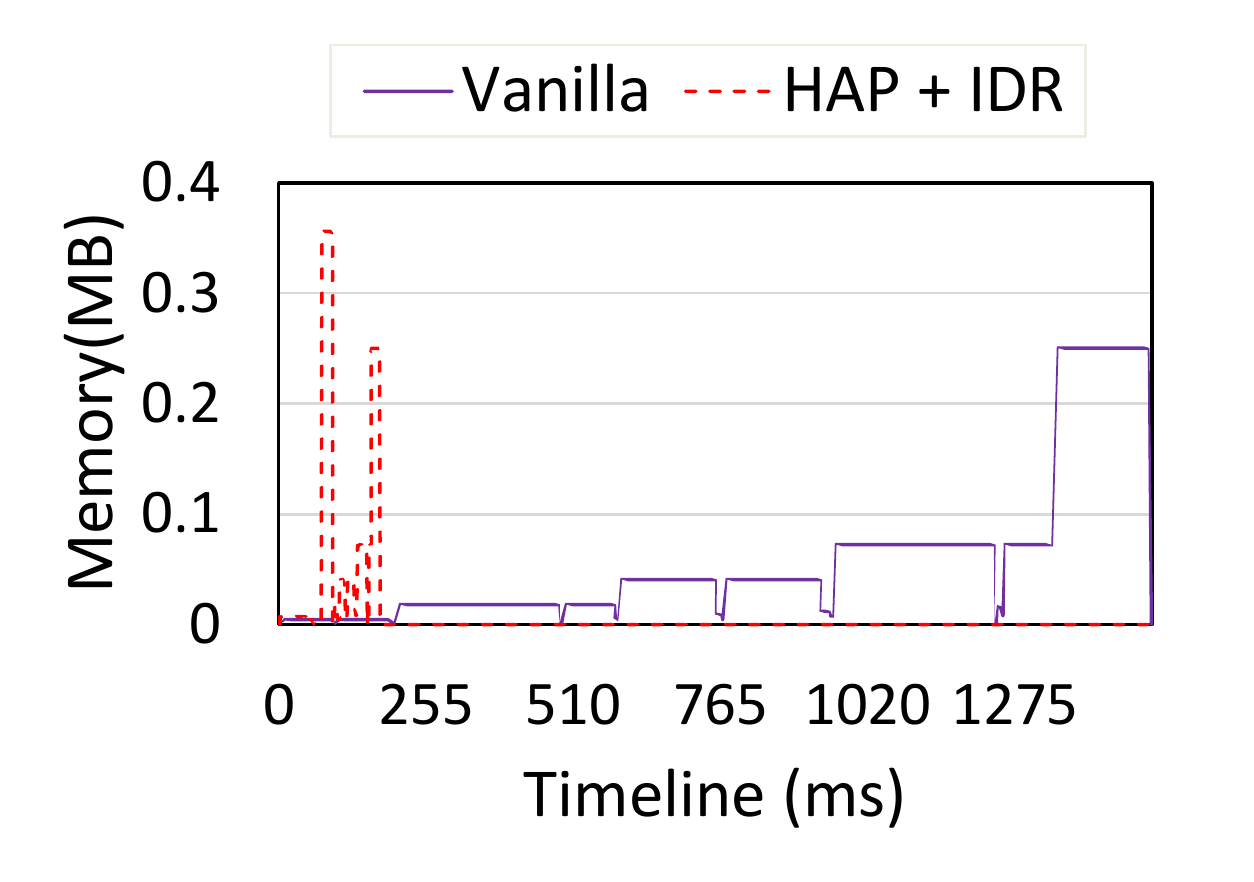}
	}
	\subfigure[SqueezeNet SRAM Cost]{
    	\label{Ssr-1} 
    	\includegraphics[width=1.6in]{./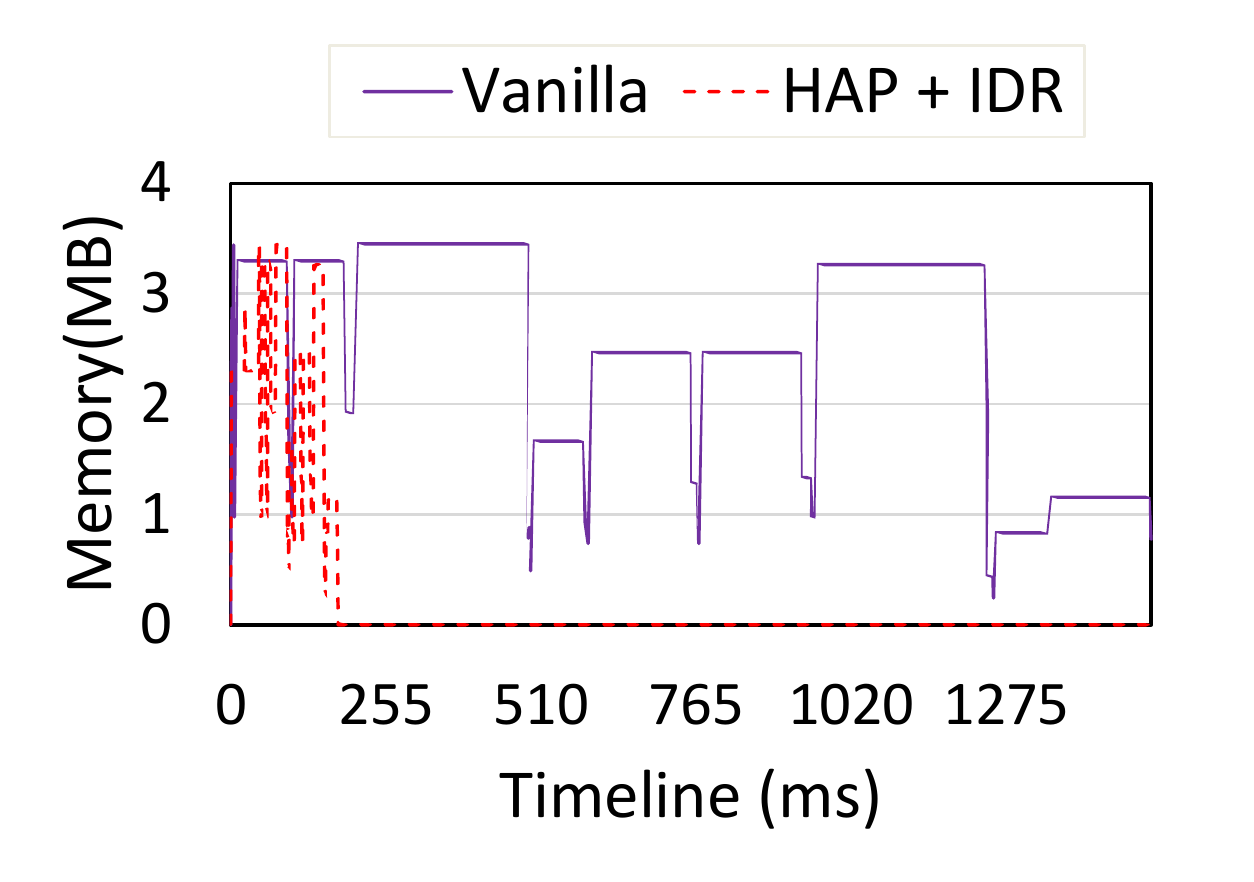}
	}
	\subfigure[SqueezeNet DDR Cost]{
		\label{Sddr-1} 
		\includegraphics[width=1.6in]{./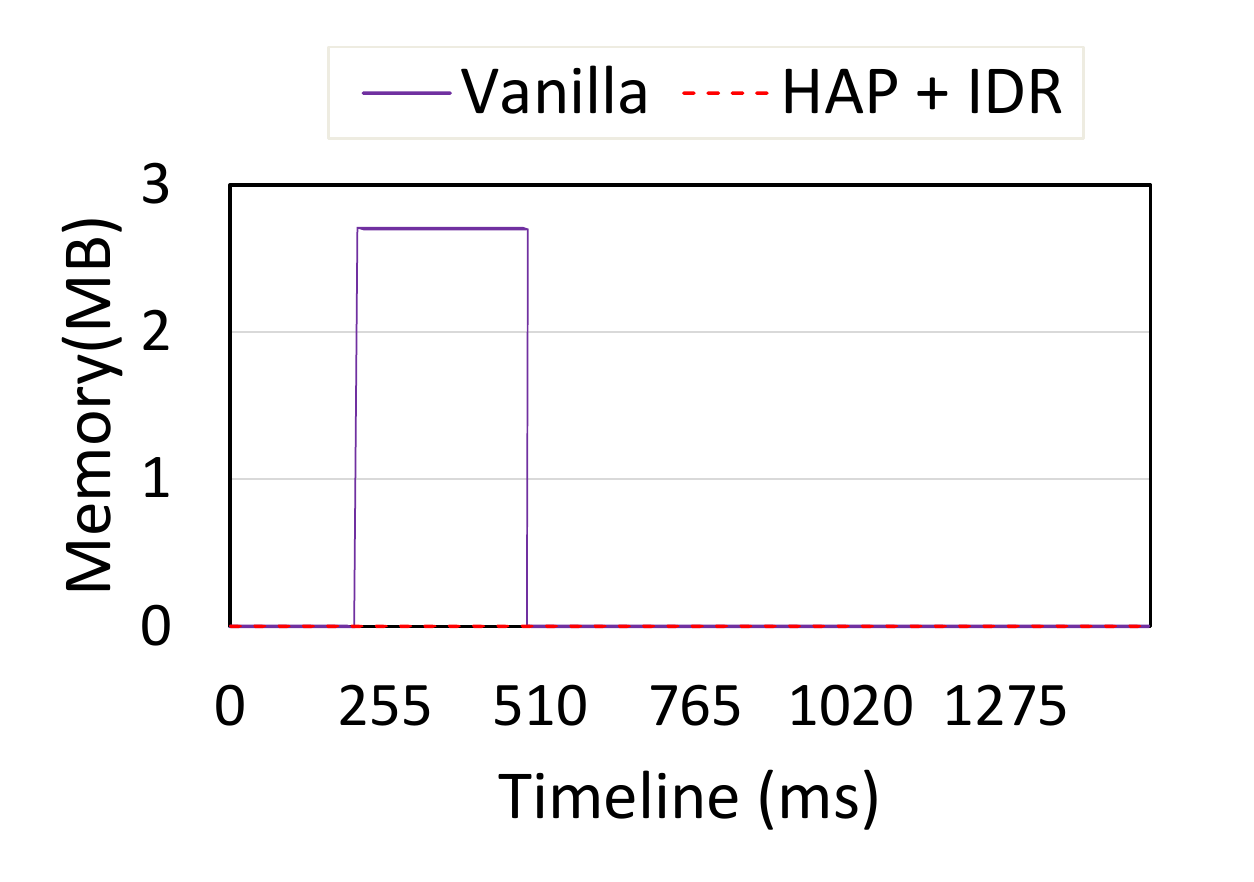}
	}
	\subfigure[SqueezeNet Total Memory Cost]{
    	\label{Stotal-1} 
    	\includegraphics[width=1.6in]{./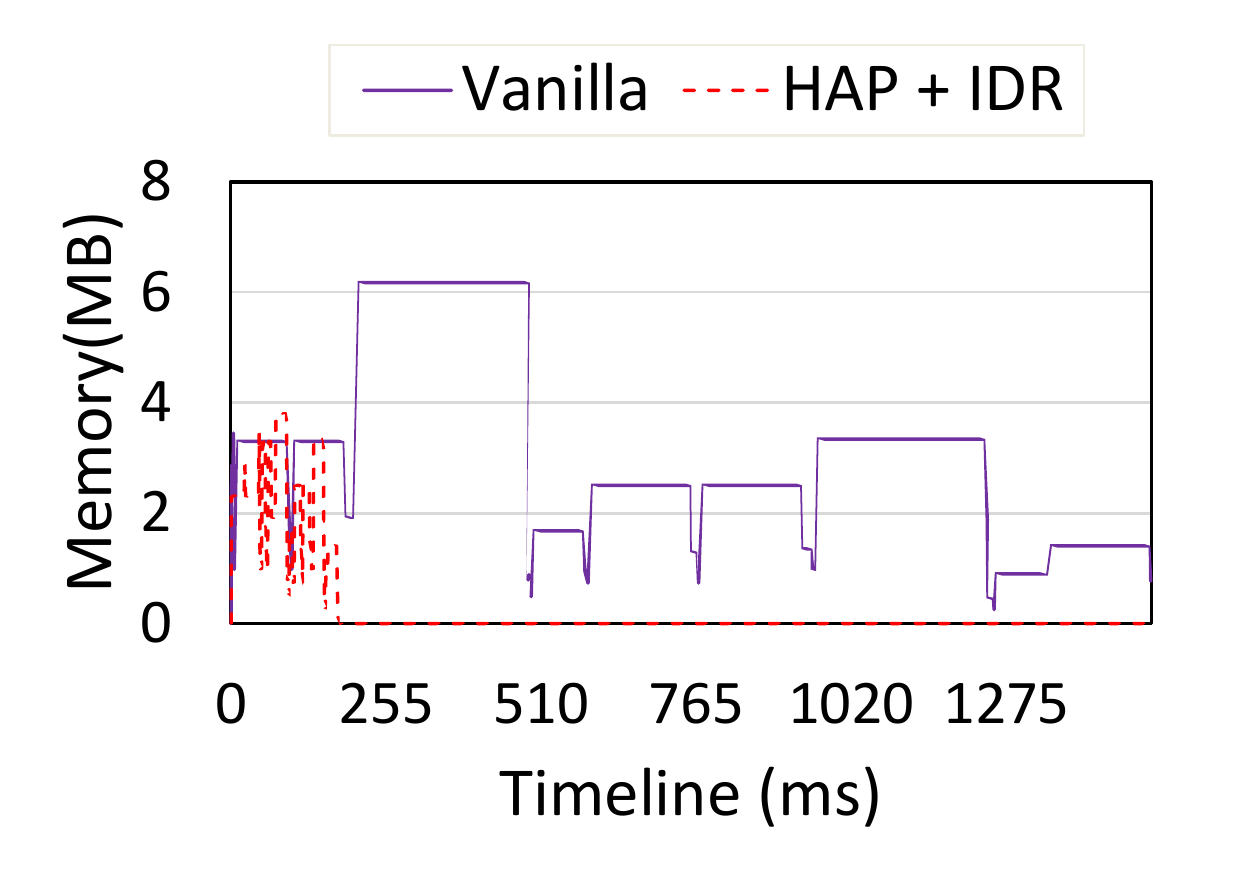}
	} \\[-2ex]
	\subfigure[ShuffleNet L2 Cost]{
		\label{ShuffleNetl2-1} 
		\includegraphics[width=1.6in]{./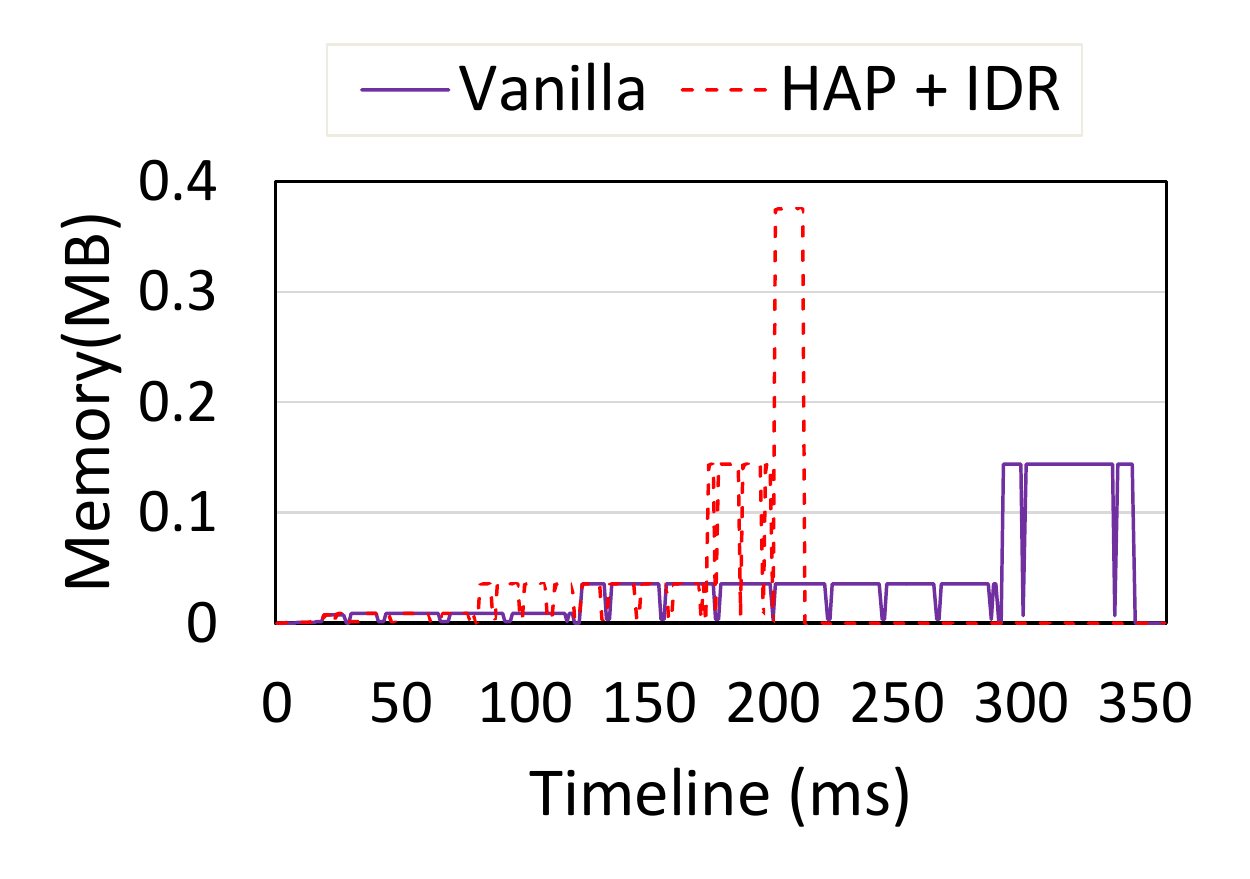}
	}
	\subfigure[ShuffleNet SRAM Cost]{
    	\label{ShuffleNetsr-1} 
    	\includegraphics[width=1.6in]{./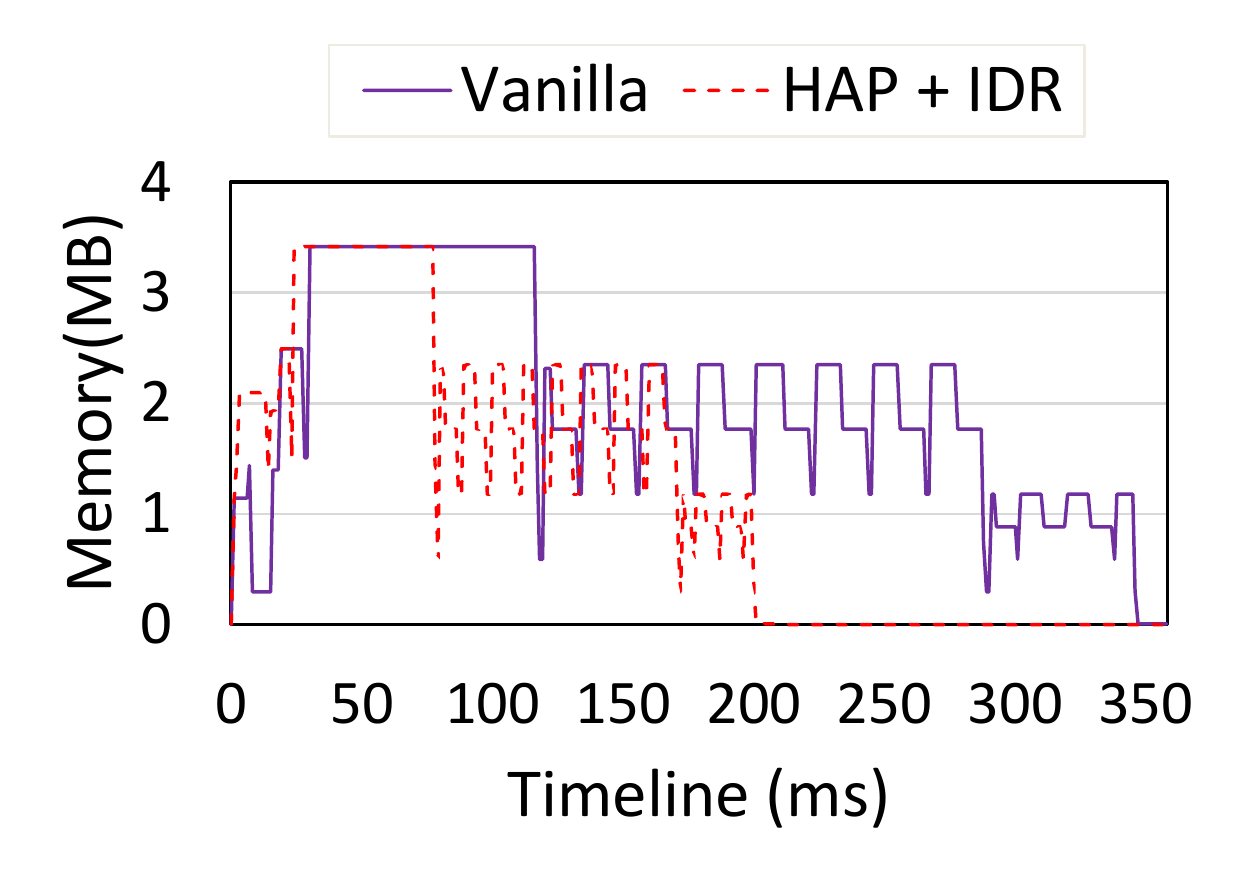}
	}
	\subfigure[ShuffleNet DDR Cost]{
		\label{ShuffleNetddr-1} 
		\includegraphics[width=1.6in]{./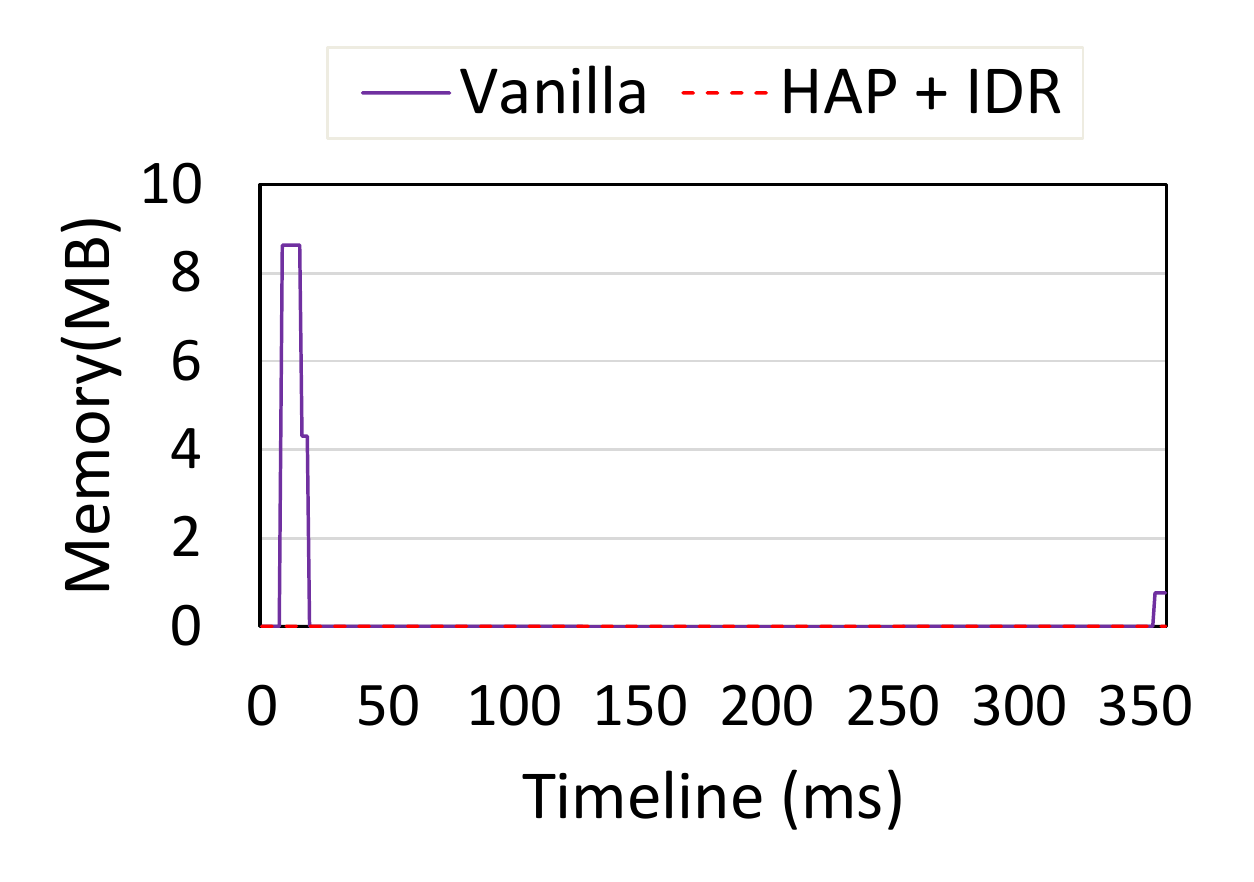}
	}
	\subfigure[ShuffleNet Total Memory Cost]{
    	\label{ShuffleNettotal-1} 
    	\includegraphics[width=1.6in]{./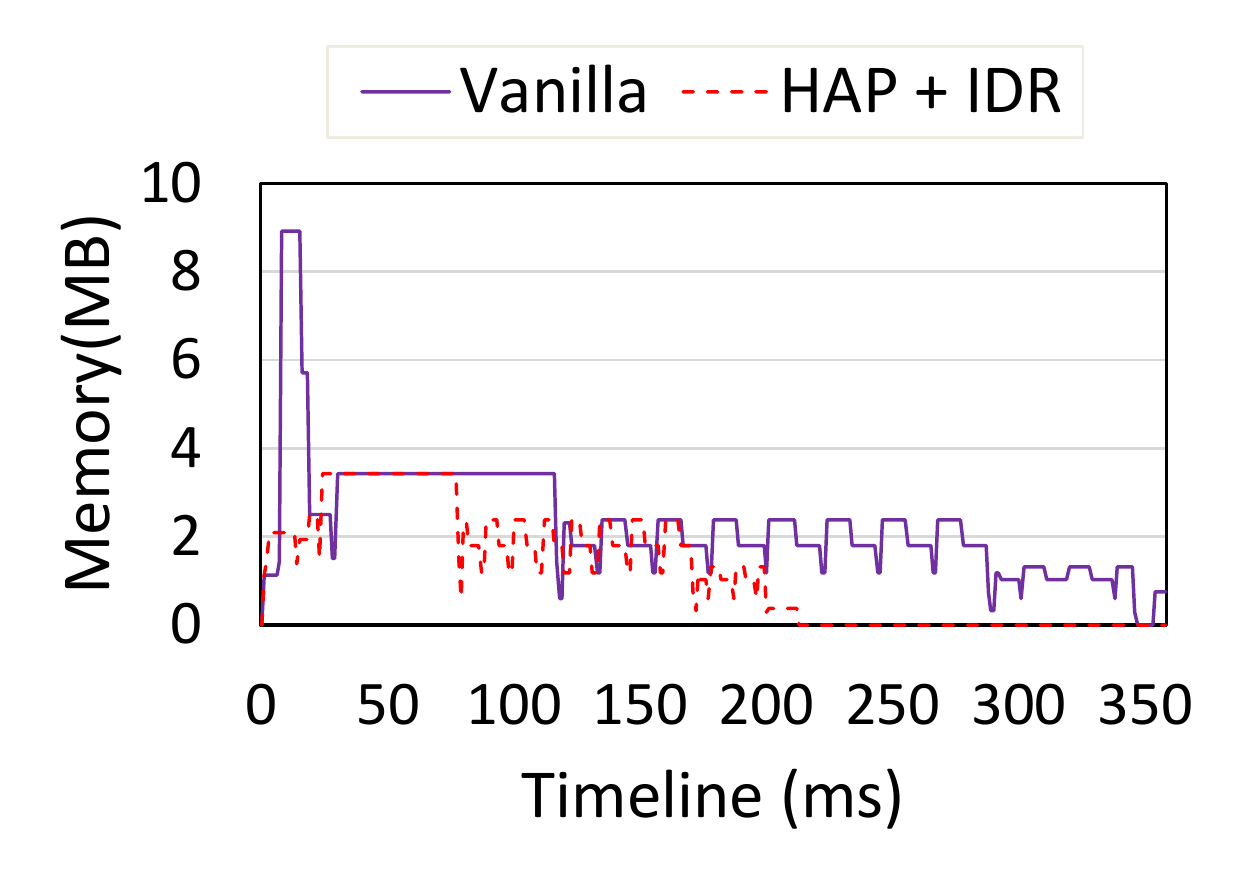}
	} \\[-2ex]
	\subfigure[CentreNet L2 Cost]{
		\label{centrenetl2-1} 
		\includegraphics[width=1.6in]{./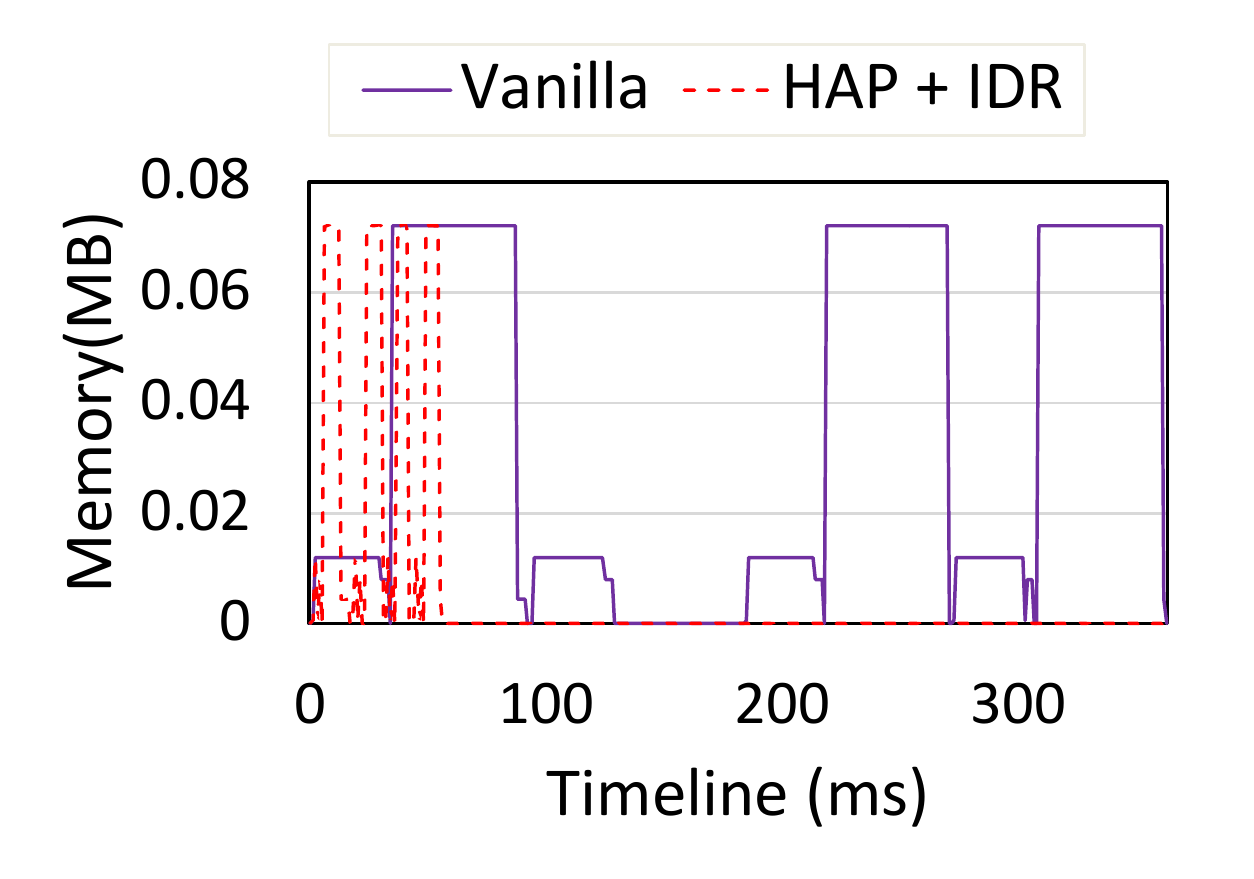}
	}
	\subfigure[CentreNet SRAM Cost]{
    	\label{centrenetsr-1} 
    	\includegraphics[width=1.6in]{./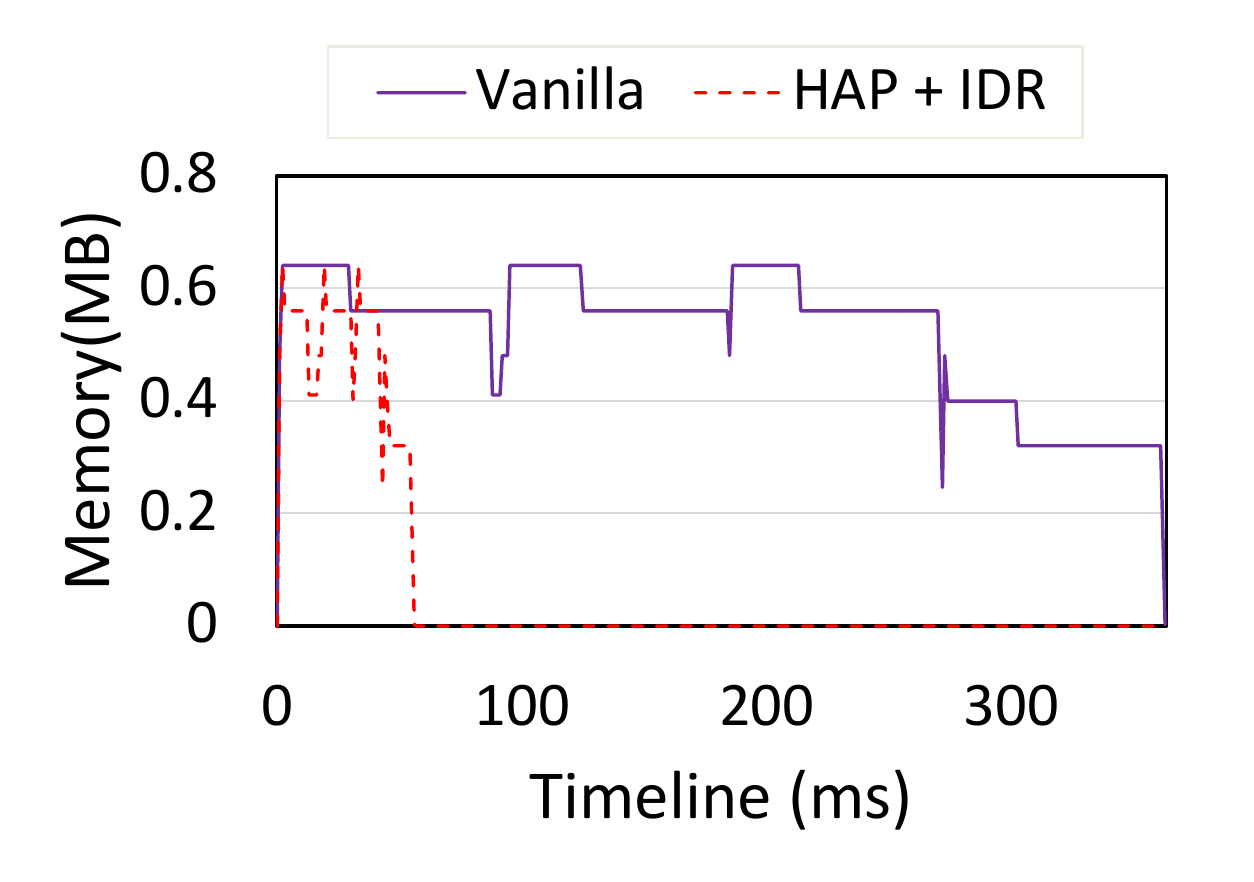}
	}
	\subfigure[CentreNet DDR Cost]{
		\label{centrenetddr-1} 
		\includegraphics[width=1.6in]{./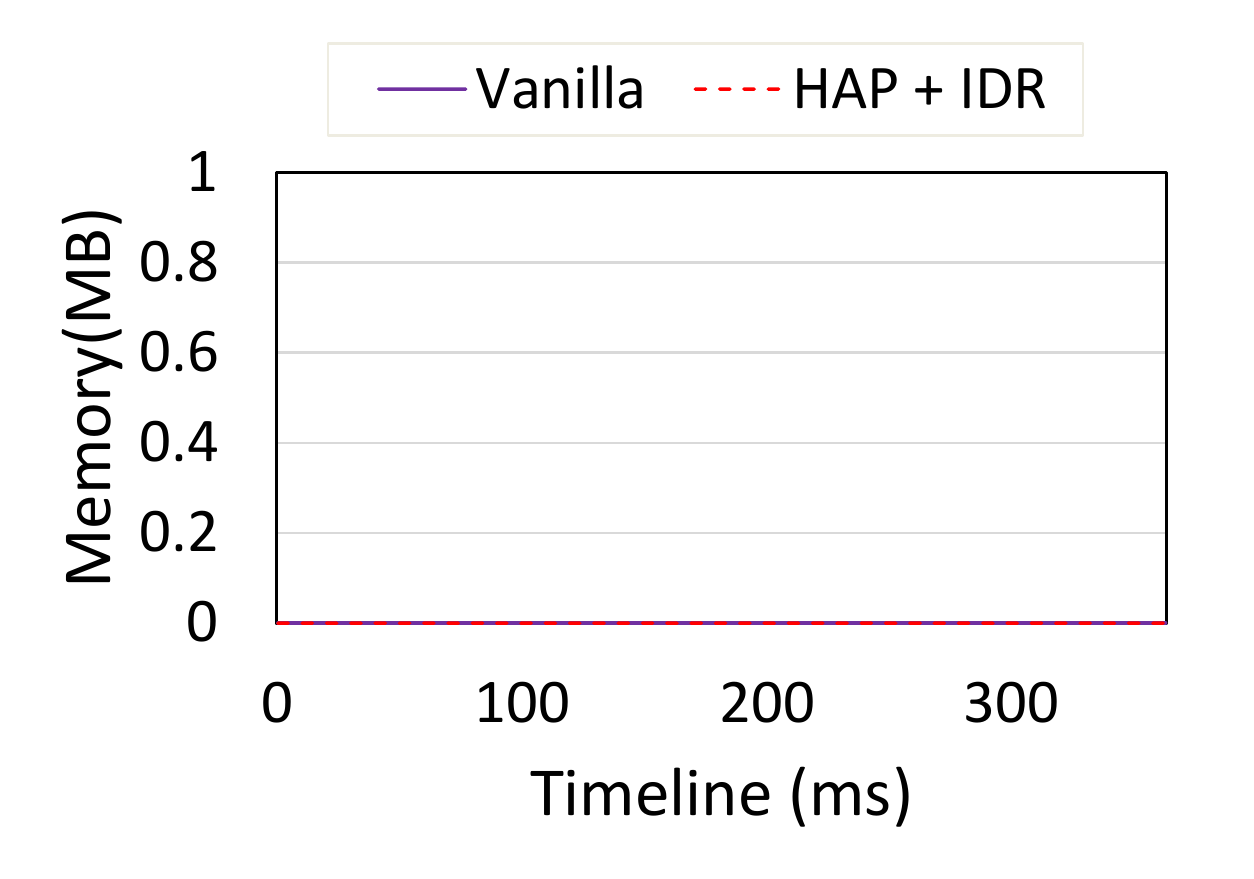}
	}
	\subfigure[CentreNet Total Memory Cost]{
    	\label{centrenettotal-1} 
    	\includegraphics[width=1.6in]{./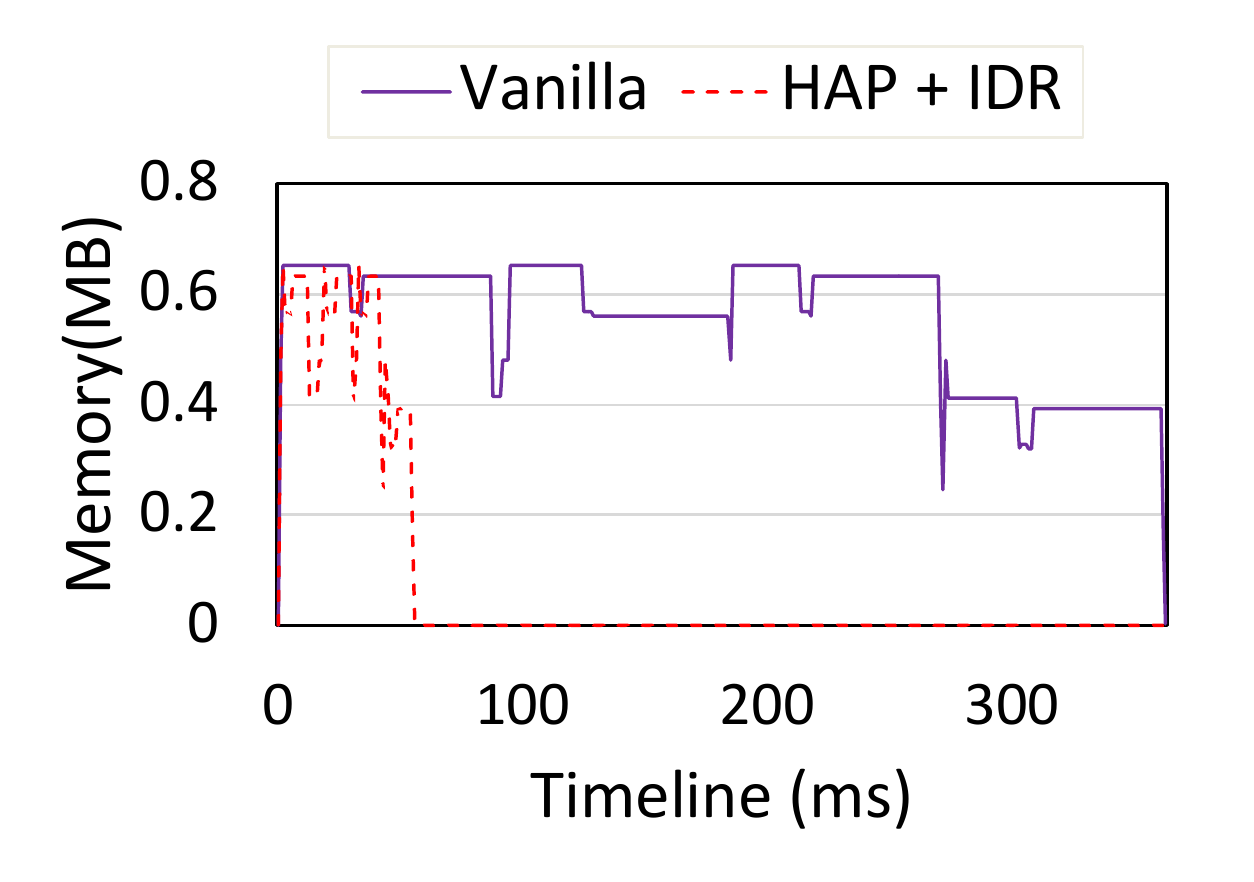}
	}\\[-2ex]
	\subfigure[Resnet18 L2 Cost]{
		\label{Resnet18l2-1} 
		\includegraphics[width=1.6in]{./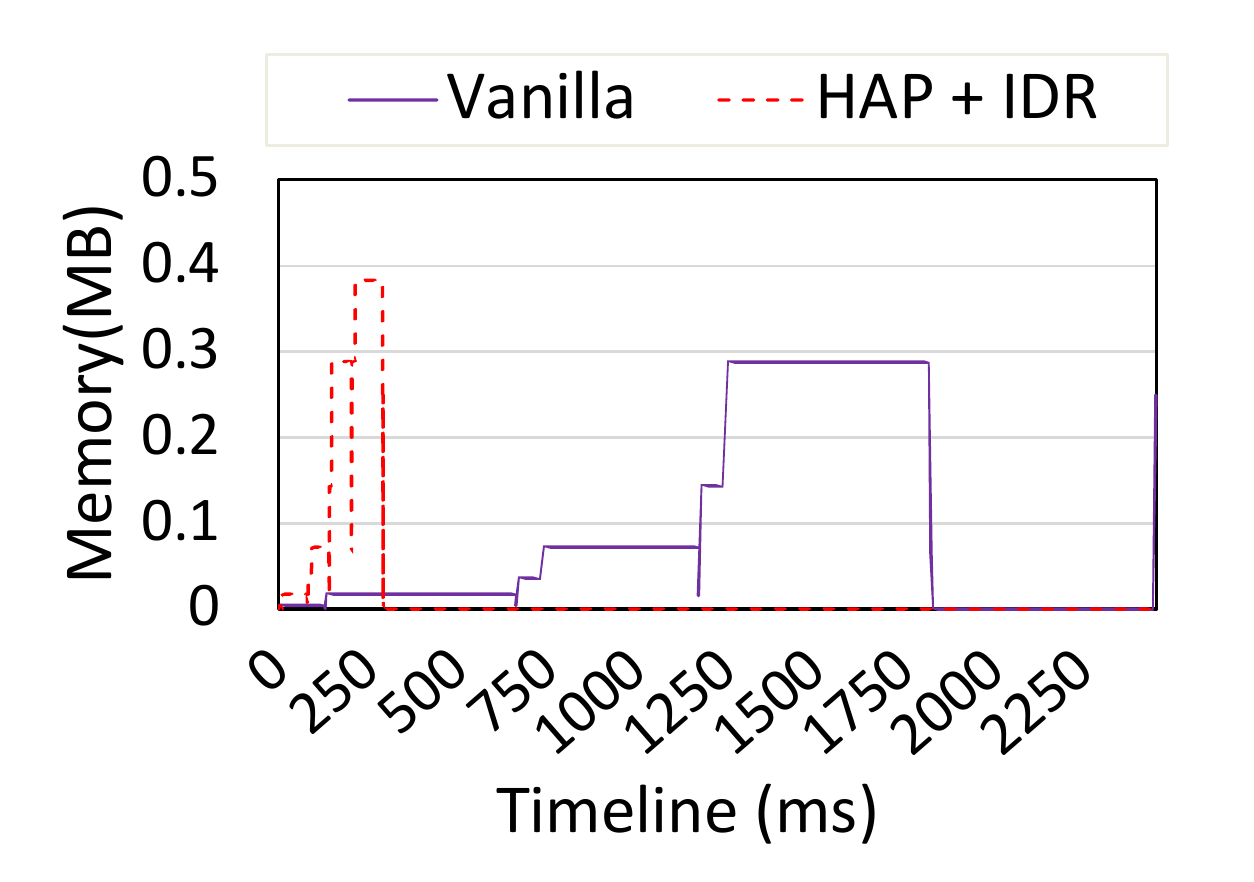}
	}
	\subfigure[Resnet18 SRAM Cost]{
    	\label{Resnet18sr-1} 
    	\includegraphics[width=1.6in]{./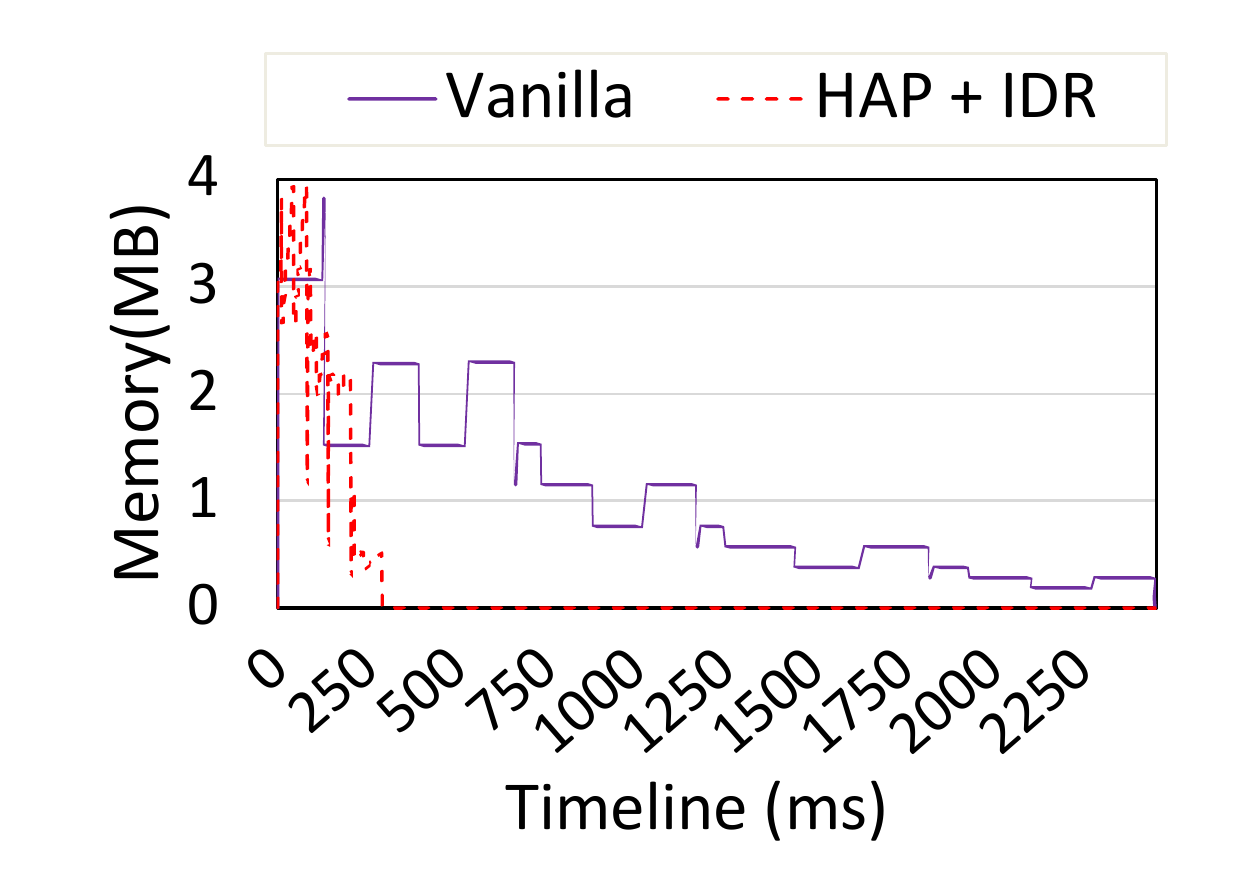}
	}
	\subfigure[Resnet18 DDR Cost]{
		\label{Resnet18ddr-1} 
		\includegraphics[width=1.6in]{./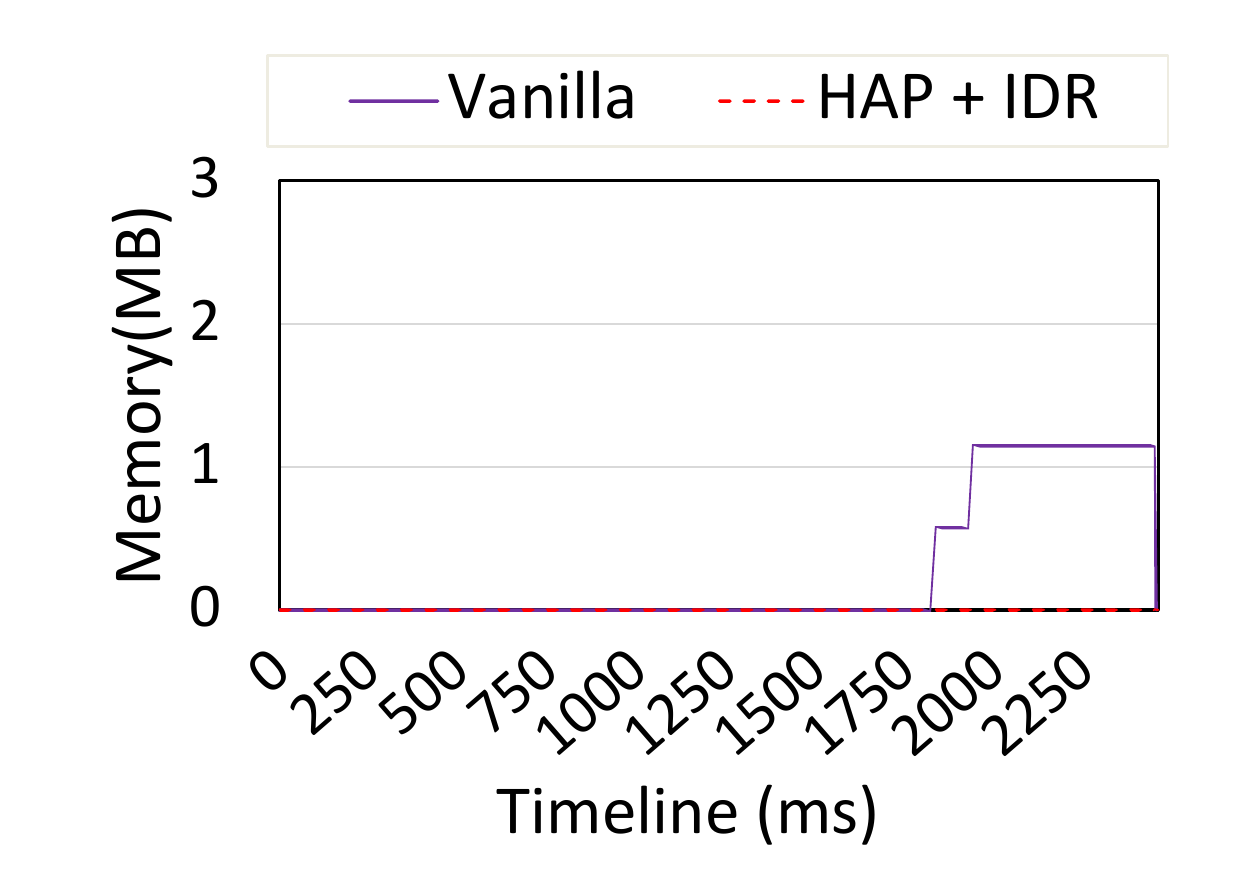}
	}
	\subfigure[Resnet18 Total Memory Cost]{
    	\label{Resnet18total-1} 
    	\includegraphics[width=1.6in]{./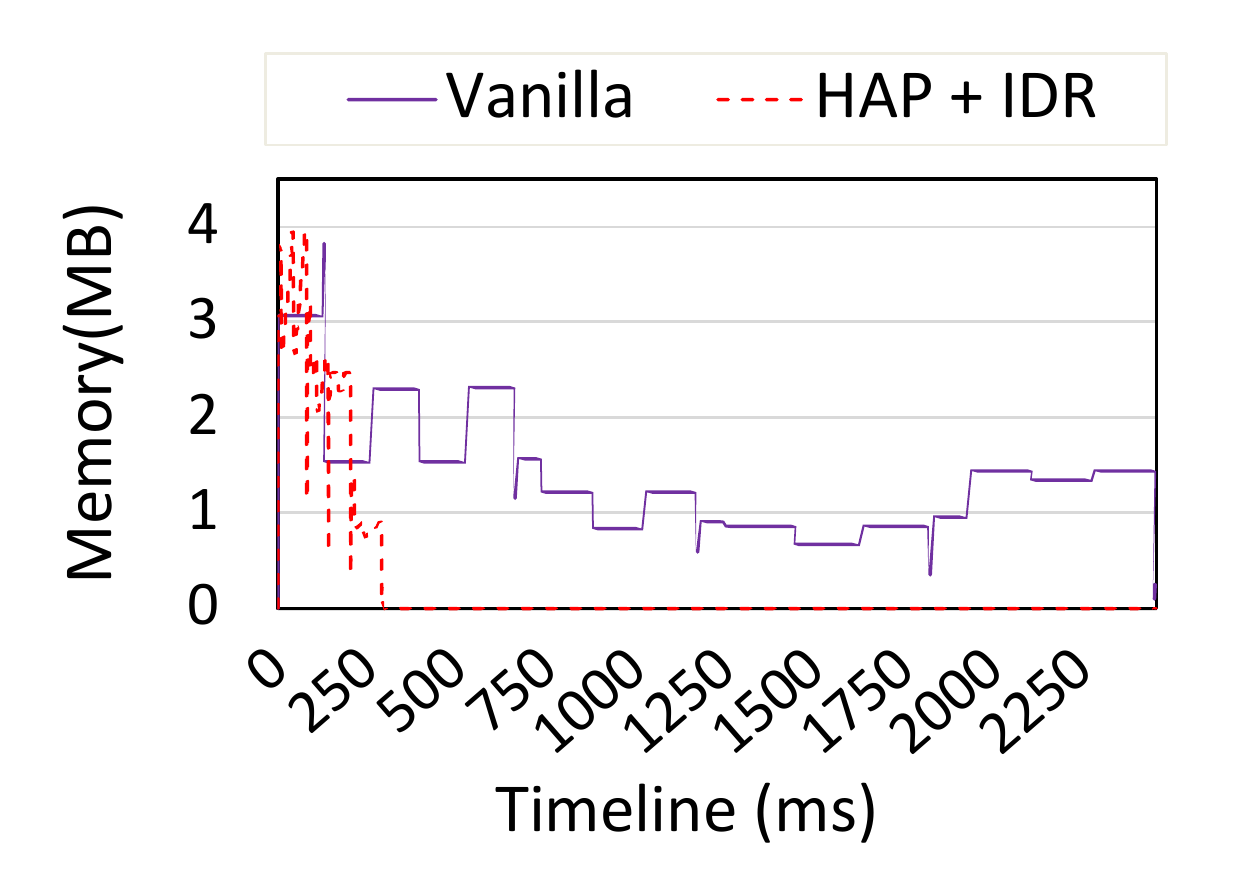}
	} \\[-2ex]
	\subfigure[LSTM L2 Cost]{
		\label{LSTMl2-1} 
		\includegraphics[width=1.6in]{./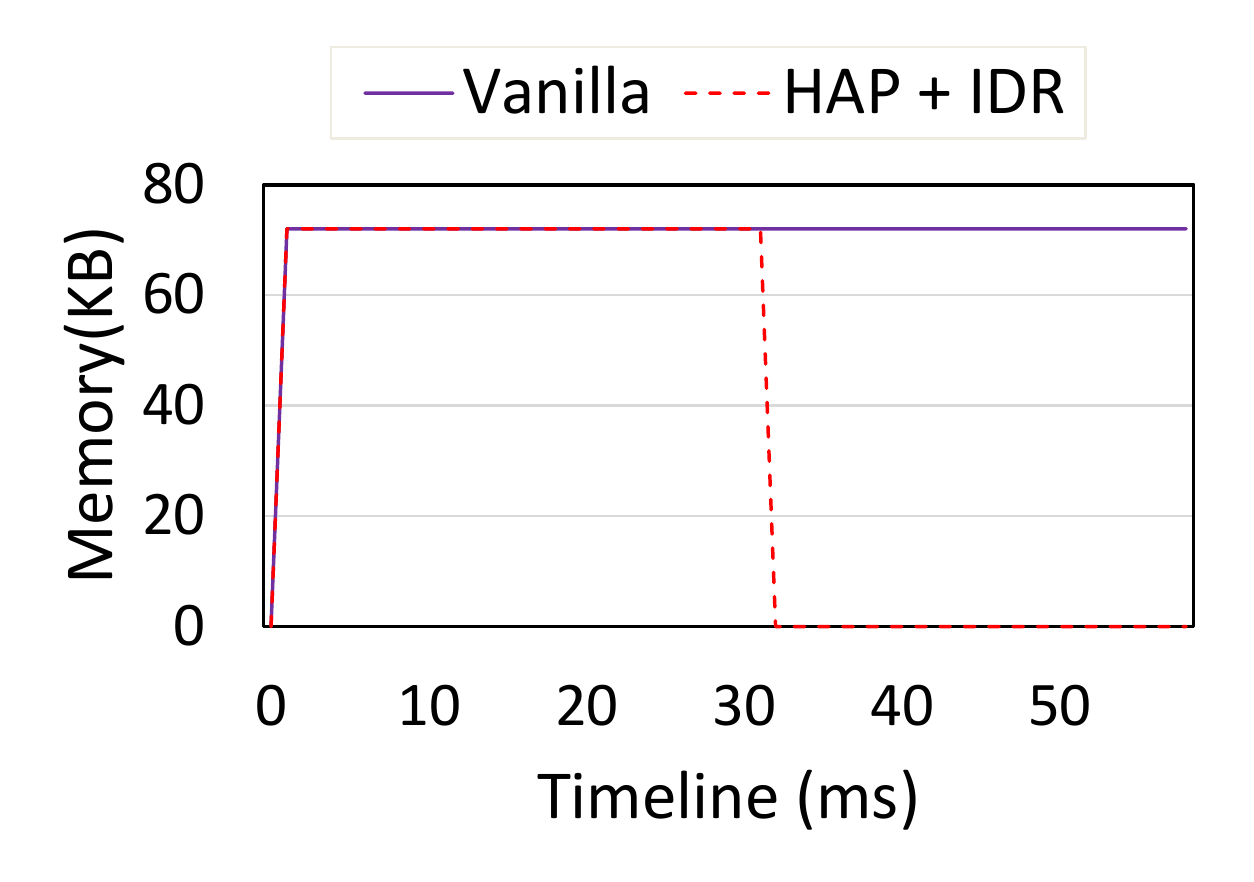}
	}
	\subfigure[LSTM SRAM Cost]{
    	\label{LSTMsr-1} 
    	\includegraphics[width=1.6in]{./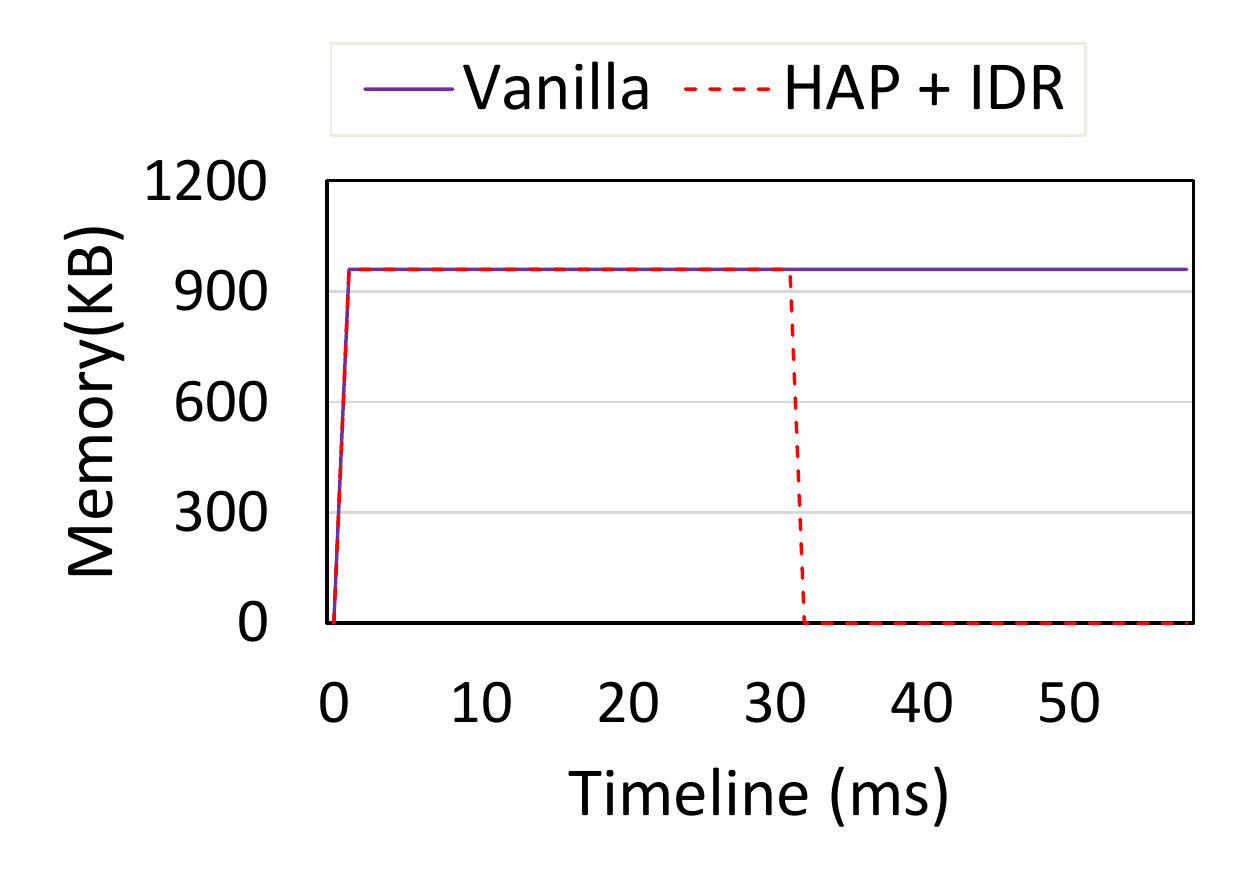}
	}
	\subfigure[LSTM DDR Cost]{
		\label{LSTMddr-1} 
		\includegraphics[width=1.6in]{./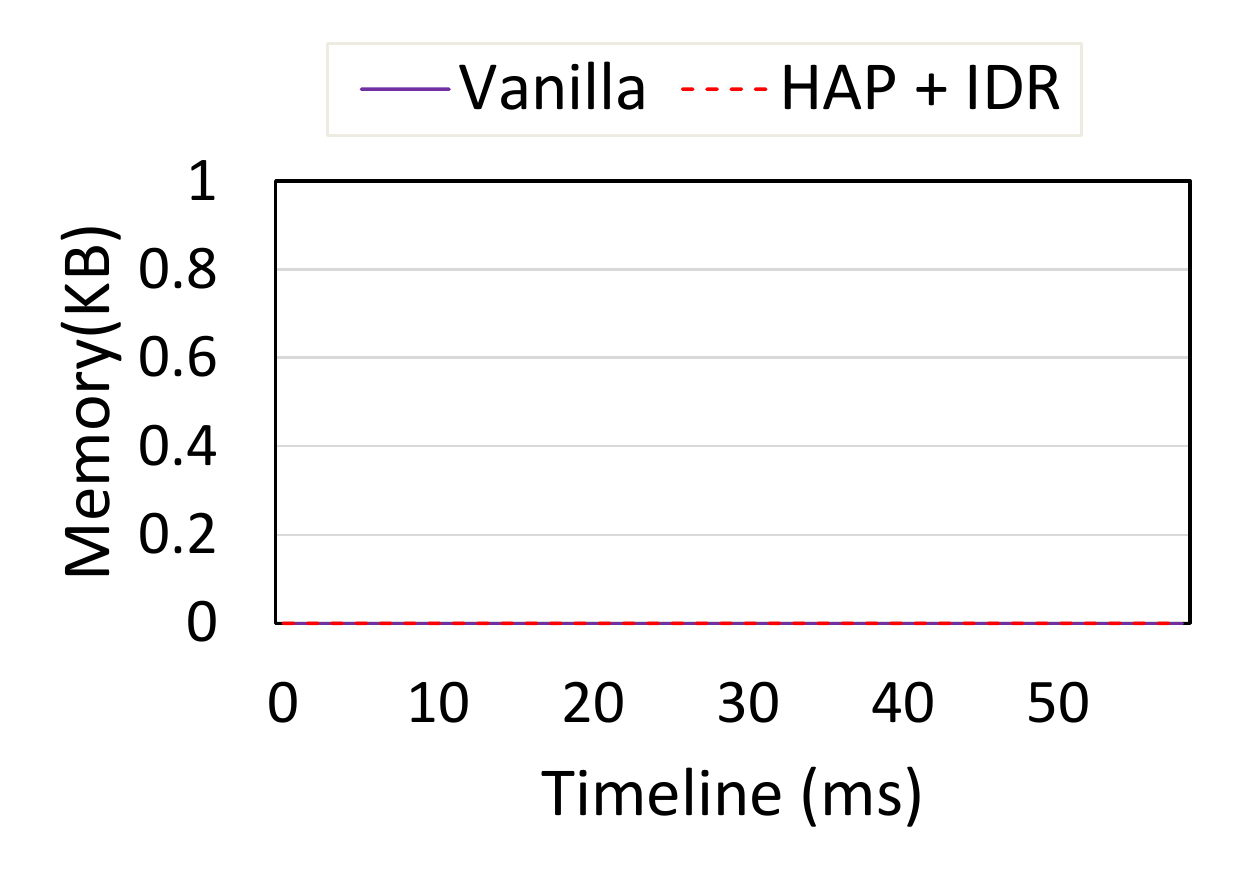}
	}
	\subfigure[LSTM Total Memory Cost]{
    	\label{LSTMtotal-1} 
    	\includegraphics[width=1.6in]{./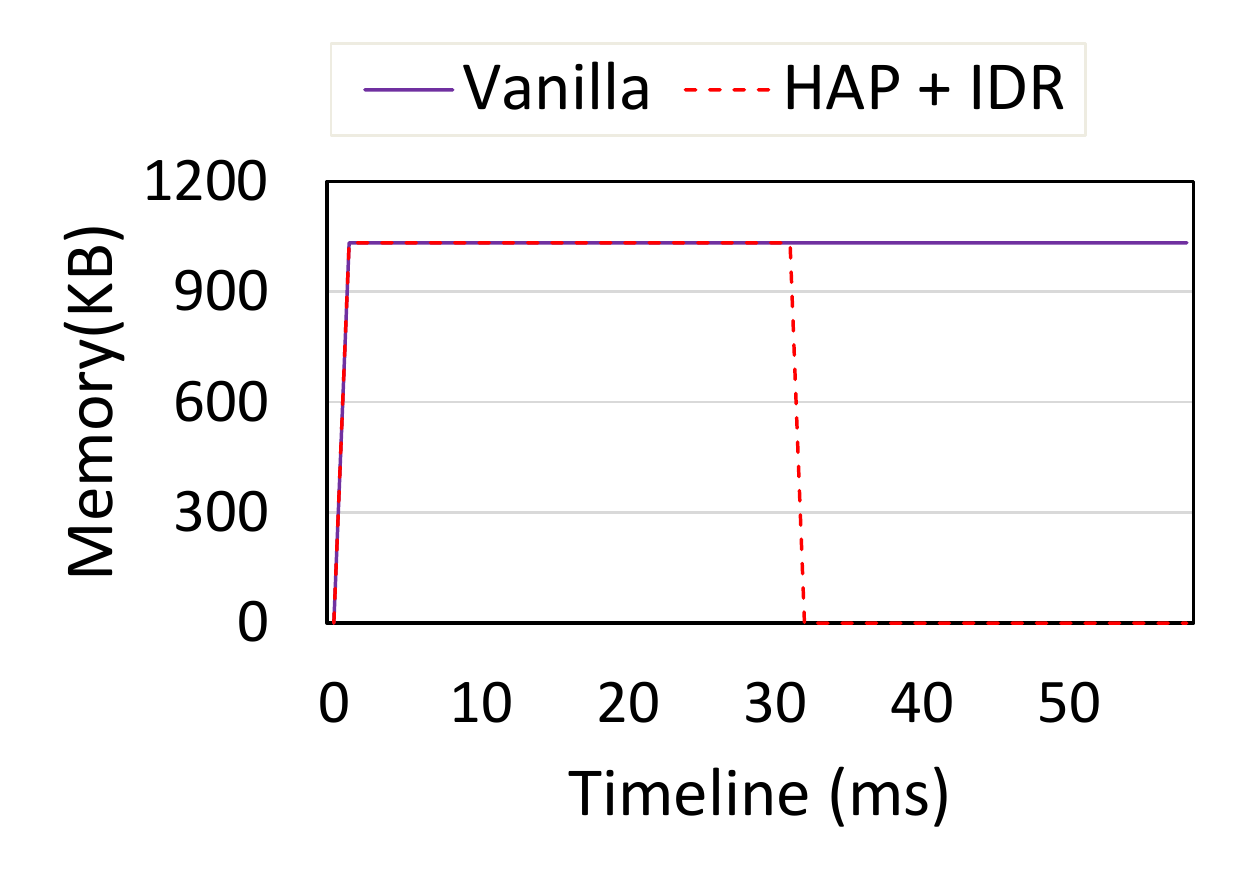}
	}
	\caption{Resources cost comparison on TMS320C6678}
	\label{MC} 
\end{figure}
\makeatletter
\setlength{\@fptop}{0pt}
\makeatother

\begin{figure}[!t]
	\centering
	\subfigure[MobileNet Resources Cost]{
		\label{FpgaMobileRc-1} 
		\includegraphics[width=2.2in]{./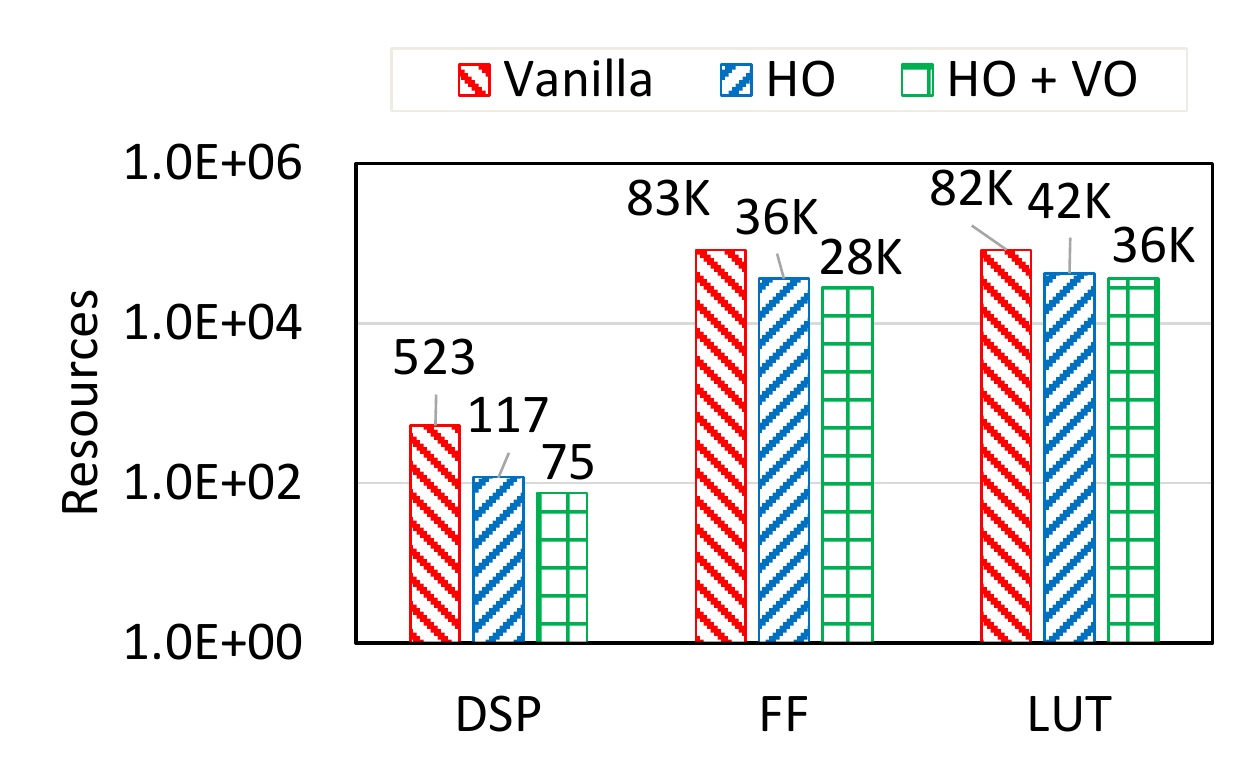}
	}
	\subfigure[ShuffleNet Resources Cost]{
    	\label{FpgaShuffleNetrc-1} 
    	\includegraphics[width=2.2in]{./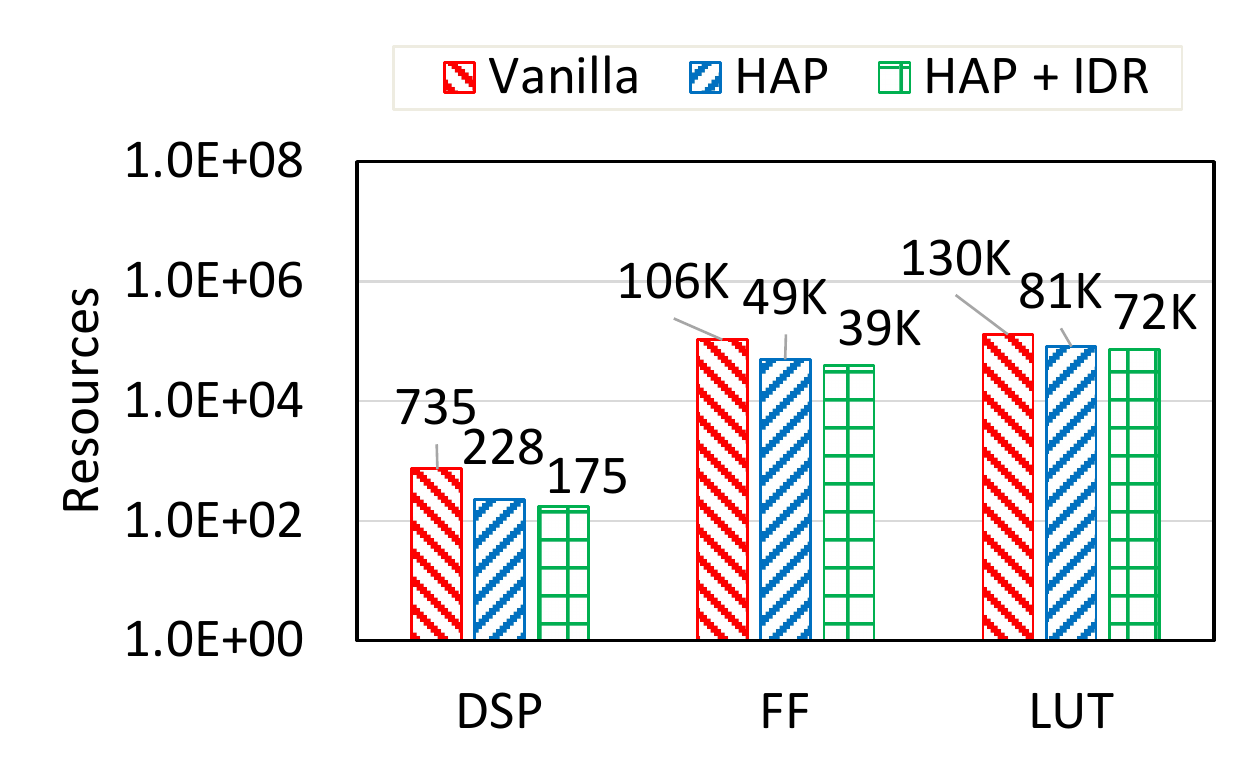}
	}
	\subfigure[SqueezeNet Resources Cost]{
		\label{FpgaSqueezeNetRc-1} 
		\includegraphics[width=2.2in]{./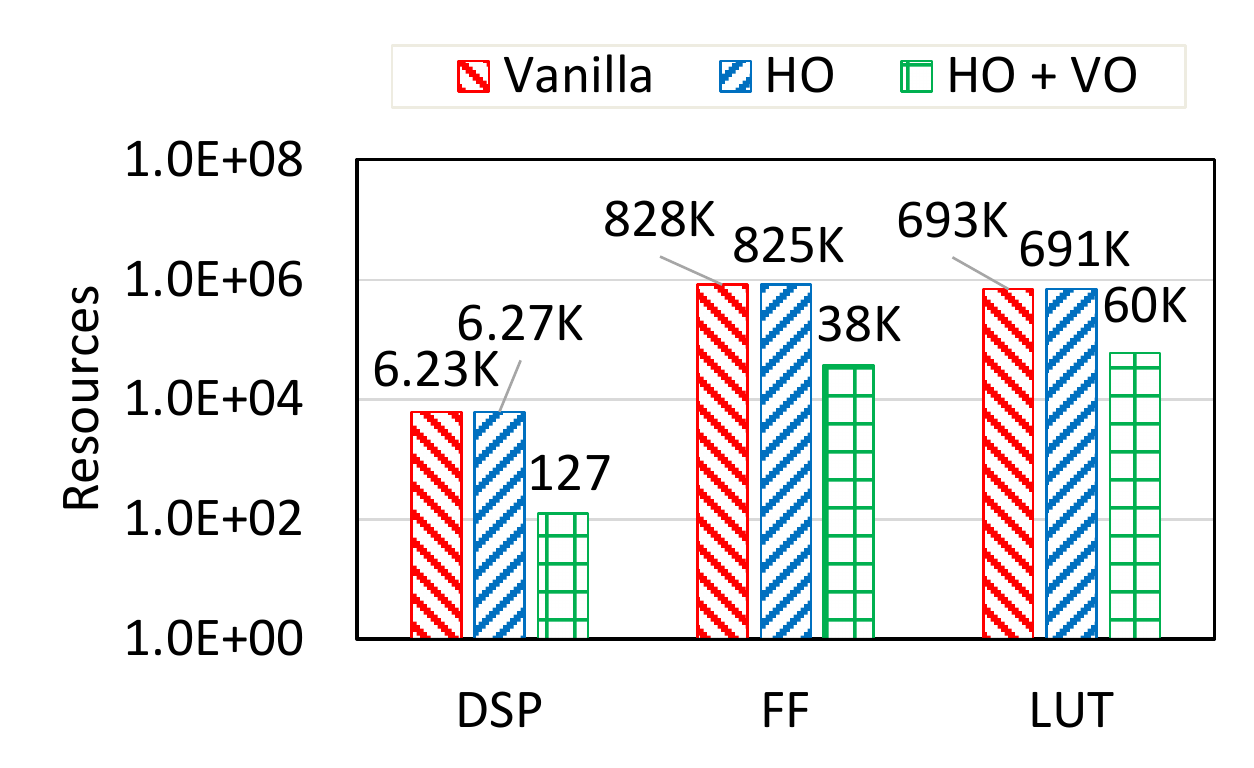}
	}
	
	\subfigure[ResNet18 Resources Cost]{
		\label{ResNet18Rc-1} 
		\includegraphics[width=2.2in]{./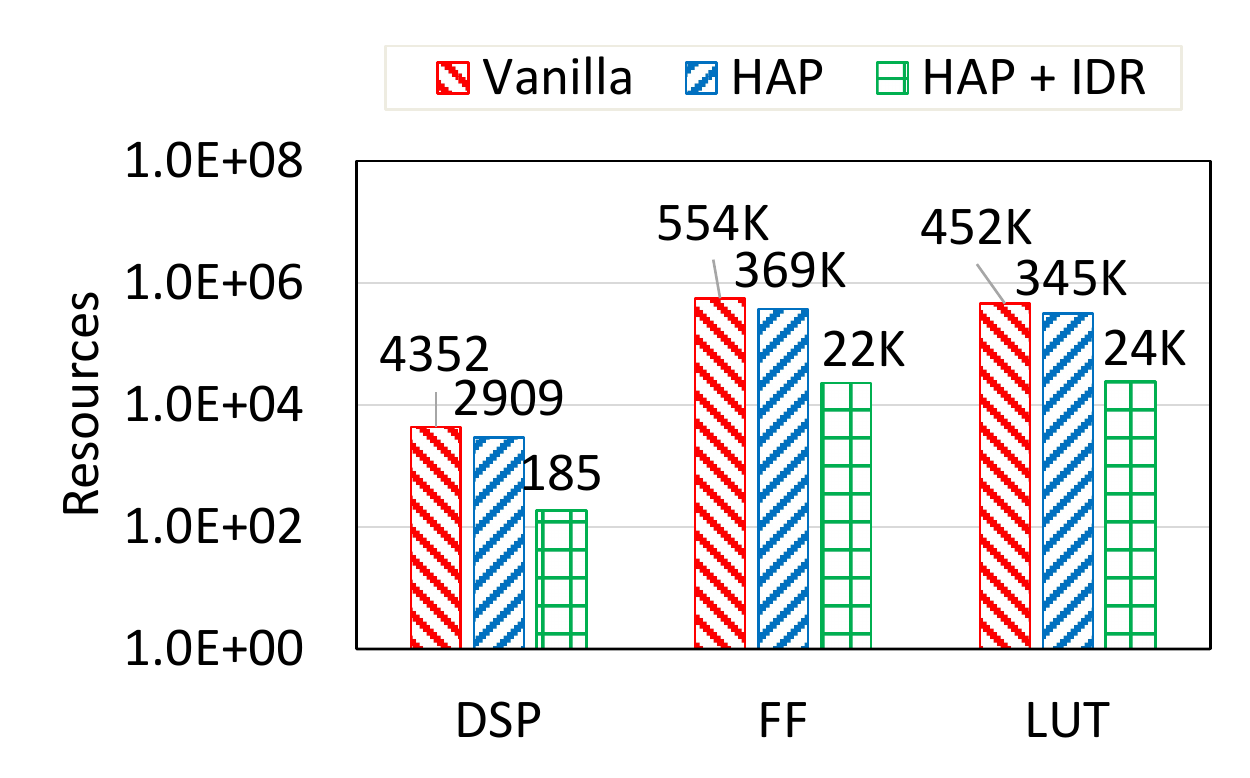}
	}
	\subfigure[LSTM/H:128 Resources Cost]{
		\label{lstmRc-1} 
		\includegraphics[width=2.2in]{./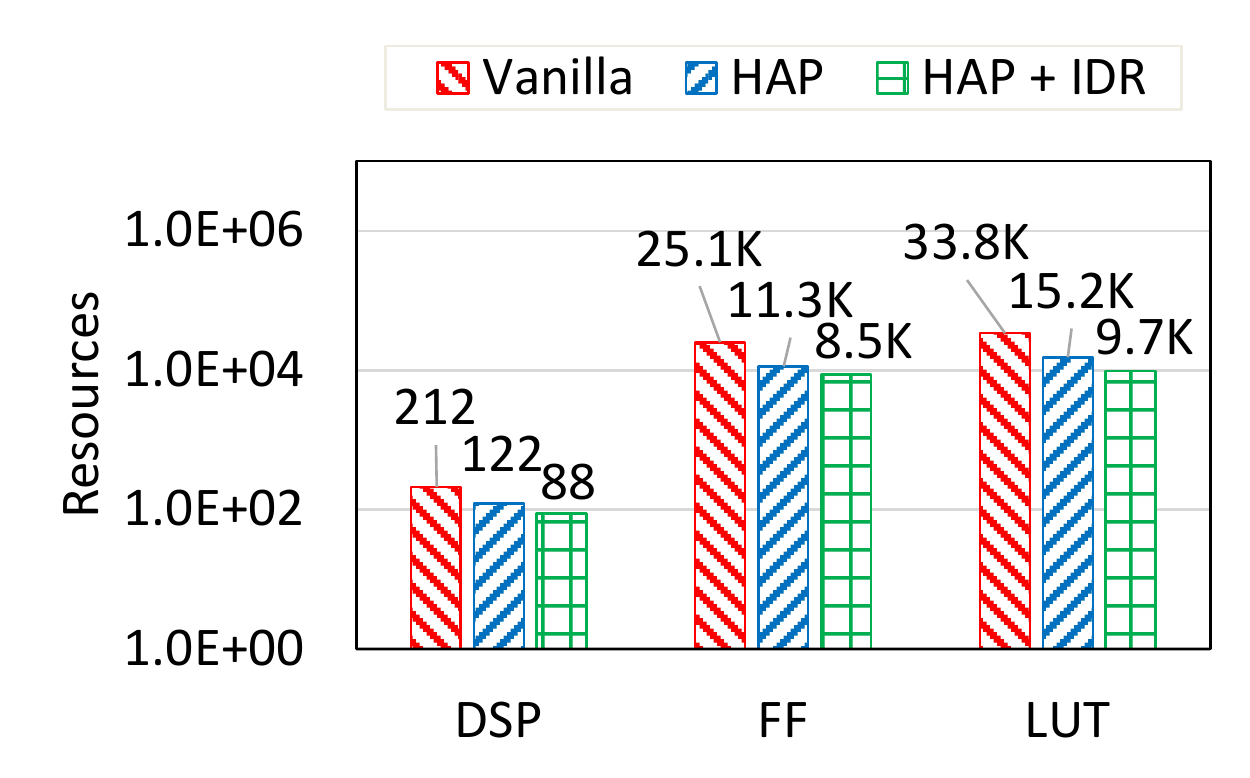}
	}
	\subfigure[CentreNet Resources Cost]{
		\label{centrenetrc-1} 
		\includegraphics[width=2.2in]{./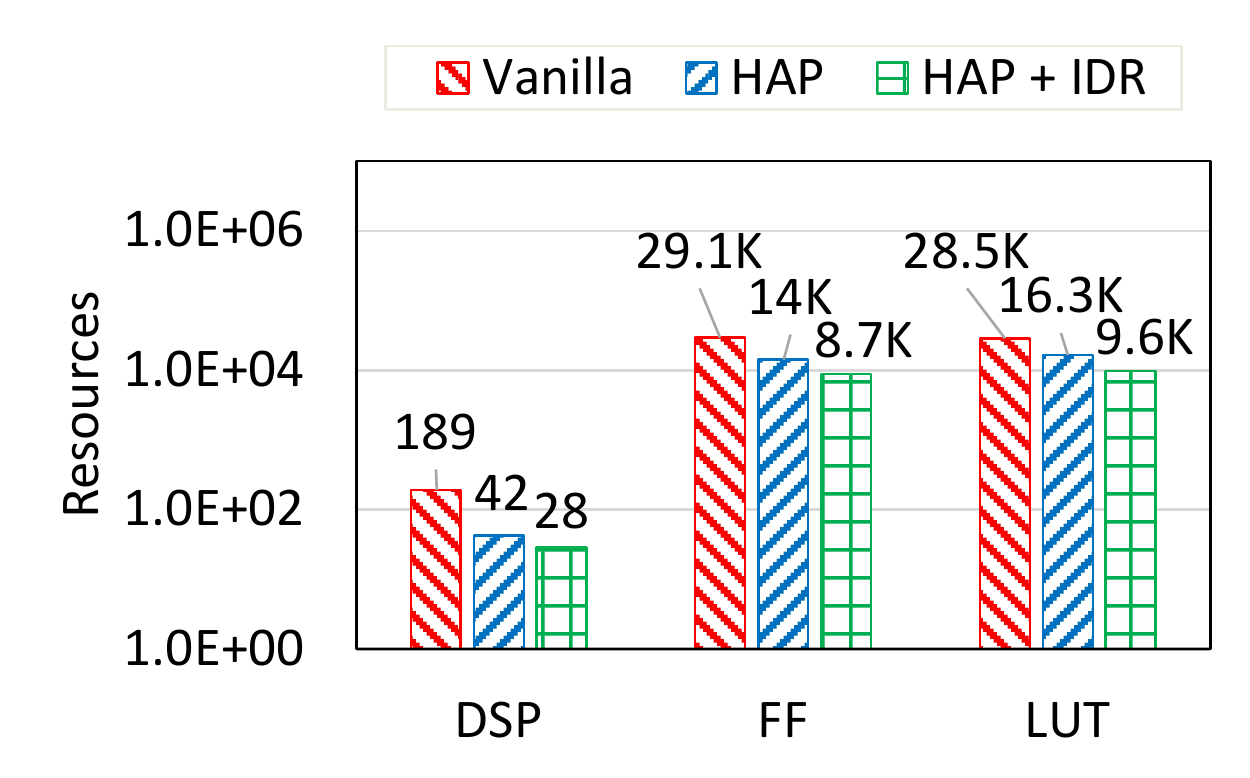}
	}
	\caption{Resources cost comparison on ZCU102}
	\label{Restructure} 
\end{figure}

% As for SqueezeNet (Figure \ref{Sl2}-\ref{Stotal}), the overheads of Vanilla's DDR mainly come from the feature map, as described in the case of MobileNet. 

% As for ShuffleNet (Figure \ref{ShuffleNetl2-1}-\ref{ShuffleNettotal-1}), the large size of feature map also causes much DDR overheads to the Vanilla baseline, but unlike MobileNet and SqueezeNet, SRAM is mostly idle (comparing the initial 30ms of Figure~\ref{ShuffleNetsr-1} with that of Figure~\ref{Msr-1} and Figure~\ref{Ssr-1}) and we can use CBS to split the feature map and put into SRAM, without introducing extra padding operations. The other part of overheads is caused by the large size of the ShuffleNet's fully-connected layer (weight parameters). Similiar to the optimization for MobileNet.  We use CBS to partition the  weight parameters of the fully-connected layer and place the partitioned parameters into L2 storage in batches. Therefore, DDR overheads are reduced and inference is further accelerated due to faster data access.

% 9 times, 0.9 * 9 =8.1 
